# Supplementary material for: The Selection Problem in Multi-Query Optimization: a Comprehensive Survey
Source: arXiv:2412.11828 source file (2025-01-25)
Supplement: Supplementary file 1 [file chapters_appendix.tex]

%\appendix

% \section{NP-Hardness Theorem}
% \label{appendix:np-hardness}

% \begin{theorem}
% View Selection Problem on binary AND-DAG under space constraints is NP-hard.
% \end{theorem}
% \begin{proof}
% Let's reduce knapsack problem to it. Suppose we have $n$ items with values $v_i$ and weights $w_{i}$ and our total space budget equals to $W$. We can assume that $\min_i(w_{i})^2 > W$, because otherwise we can do so by scaling with an appropriate constant. Consider a join of $n$ tables with independent $\sigma_i$ WHERE-clauses whose size are $w_i + v_i$ and $w_i$ before and after filtering, respectively. If the time of reading and filtering table $\{T_i\}_{i=1}^{i=n}$ is equal to its size, then under \textit{any} execution plan of $q$ the View Selection Problem is equivalent to the selection of items in the knapsack problem. Indeed, we can only select candidates that correspond filtered table ($c_i=\sigma_i(T_i)$). Any other candidate in the graph will have size at least $\min_i(w_{i})^2$, and this violates space constraints. The benefit we get from selection $c_i$ is equal to 
% $$
%     \underbrace{(w_i + v_i)}_{\text{compute $c_i$ }} - \underbrace{w_i}_{\text{reread $c_i$ }} = v_i,
% $$
% which is entirely consistent with the selection of the item $i$.
% \end{proof}

% \section{Compressed Expression Forest}
% \label{appendix:compression}


% Here we show how we can implement the optimisation proposed in Chapter \ref{chapter:applying} on an arbitrary subset of selected candidates without traversing the whole expression forest. That is interesting, because in practice we can limit the search for optimal usage of candidates only to those of them that were selected in the first step of the iteration (otherwise candidates cannot be reused). It means that the set of candidates considered by the ILP solver at each iteration can be much smaller than the size of the whole expression forest, so we have to take it into account for a fair comparison of the proposed optimisation.

% \begin{figure}
%   \centering
%   \includesvg[width=0.6\linewidth]{pictures_compression}
%   \caption{To keep only the selected candidates from the expression forest $\mathcal{F}$ and still preserve the topological order between them, we can represent them as a compressed forest $\mathcal{F}'$. Here, selected candidates are represented by gray nodes, and unselected ones by white. The operation nodes have been removed for simplicity.}
%   \label{fig:compression}
% \end{figure}

% The key observation is that the only requirement for the query representation used by our proposed optimization is that the topological order of the candidates must be \textit{maintained}. So, we can compress expression forest to include only the current set of selected candidates. An example of such compression is depicted in Figure \ref{fig:compression}. The only difficulty is that the set of selected candidates \textit{changes} at each iteration. So, we have to \textit{rebuild} our compressed forest too. The updating in the case of removing a candidate is straightforward — we simply move the edges from the removed vertex to its parent. Adding a new candidate, however, requires consideration of the topology induced by the complete expression forest, which is unfortunately no longer represented after compression. A pivotal observation for addressing this challenge is that an edge $parent \rightarrow child$ in the compressed forest exists only if $parent$ is the lowest ancestor of $child$ among all selected candidates. Moreover, we need to add the edge $c_{new\_child} \rightarrow c_{old\_child}$ only to those vertices that either lack a parent or whose lowest ancestor is also the lowest ancestor to $c_{new\_child}$. Answers to all requests of the type $is\_parent(x, y)$ can be precomputed in quadratic time (on the size of \textit{original} expression forest), so that we can get them later in $O(1)$ time. Then by traversing the vertices from top to bottom and confirming that $is\_parent(x, c_{new\_child}) = True$, we can identify all lowest ancestors $c_{parent}$ and subsequently all $c_{old\_child}$ nodes. This procedure is depicted in Figure \ref{fig:rebuilding}. As result,  the total running time of our proposed solution to add / remove \textit{one} candidate is no more than linear on the number of selected candidates.

%satisfying $lca(child, x) = x$.\footnote{$lca(x, y)$ denotes the lowest common ancestor of vertices $x$ and $y$.} Moreover, we need to add the edge $c_{new\_child} \rightarrow c_{old\_child}$ only to those vertices that either lack a parent or whose lowest ancestor is also the lowest ancestor to $c_{new\_child}$. By traversing the vertices from top to bottom and confirming that $lca(c_{new\_child}, x) = x$, we can identify $c_{parent}$ and subsequently all $c_{old\_child}$ nodes. This procedure is depicted in Figure \ref{fig:rebuilding}. 

%Note, that in general in the case of DAG $lca(x,y)$ is a \textit{set} of vertices, and instead of using equality we should check if the element \textit{is included} in the set on lowest common ancestor\textit{s}. In paper \cite{bender2005lowest}, it was shown that in cubic preprocessing time we can prepare a lookup table for processing $lca(x,y)$ requests in $\mathcal{O}(1)$ time. So the total running time of our proposed solution to add / remove one candidate is no more than quadratic\footnote{on average, due to the use of hash set}.


% \begin{figure}
%   \centering
%   \includesvg[width=0.6\linewidth]{pictures_rebuild}
%   \caption{In order to add a new candidate $c_4$ to the set of selected candidates $\{c_1, c_6, c_7, c_8\}$, the compressed forest $\mathcal{F}'$ needs to be rebuilt. For this purpose, it is sufficient to first find a parent $parent$ for it, which turns into a search for the lowest vertices $x$ with a satisfying equation $is\_parent(x,c_4)=True$ (node $c_8$). After that, it is necessary to change the edges of all their children $y$ that satisfy the equation $is\_parent(c_4, y)=True$ (node $c_1$).}
%   \label{fig:rebuilding}
% \end{figure}
